# Supplementary material for: A Model-Based Approach to Anomaly Detection Trading Detection Time and False Alarm Rate
Source: arXiv:2006.08811 source file (2020-06-15)
Supplement: Supplementary file 1 [file appendix.tex]

\begin{appendix}

\subsection{Bucket algorithm: closed-form expressions for mean time to absorption}

\label{app:closdform}

\subsubsection{Motivation}

Sequential probability ratio test~\cite{jung2004fast} and the bucket algorithm~\cite{AvritzerBGTW06} are used to detect attacks in networks.  Their analysis involves a random walk birth-death process.  In the bucket algorithm, for instance, the initial state is a state where all buckets are empty, and the final state is a state where all buckets are full.  Understanding the mean time to reach the final state, one can tune the number of buckets and the depth of each bucket in a principled way. 
%
%In this appendix, we present some preliminary ideas on the principled tuning of the bucket algorithm.  We envision that those preliminary ideas can be combined with recent advances in the study of birth-death processes (e.g.,~\cite{jouini2008moments}) to yield more refined results.
%
In what follows, we indicate that simple algorithms to detect attacks, such as the bucket algorithm, can be tuned using first principles.

\subsubsection{Goals}

How does the depth of the bucket impact the probability of false positives?  The larger the depth of the bucket, the lower the false positive probability, but the longer it takes for a true positive to be identified.

To simplify analysis, we work under the assumption that attacks will change the response time distribution, and will always be detected.  However, the number of samples to detect the attack may vary depending on the depth of the bucket.   As our second key simplifying assumption, we assume that the number of samples to detect the attack is much smaller than the number of samples collected before getting a false positive (which should be always the case in practice: the time until a false positive should be much longer on average than the time until a true positive).  

Then, we aim at answering the following question: what is the smallest bucket depth to produce a false positive probability bounded by a given threshold?

\subsubsection{Single bucket case ($K=1$)}

We note that the bucket algorithm with a single bucket corresponds to an M/M/1 queue in discrete time.  Time is measured in number of collected samples, i.e., we consider a discrete time system where each time slot corresponds to the duration between two sample collections.  Let $1-p_1$ be the probability that a sample adds a ball into the bucket, and
\begin{equation}
    \rho_1=\frac{1}{p_1}-1.
\end{equation}
Let $V_D$ be the mean time to reach state $D$ starting from state $0$. Then, $V_D$ is given by first passage time arguments (see Section 2.5.3 in~\cite{zukerman2013introduction}),
\begin{align}
    V_D &= \sum_{n=1}^D U_{n-1}  \\
 &=    \frac{ \rho_1+1}{(1-\rho_1)\rho_1^D} \left(\frac{1-\rho_1^{D}}{1-\rho_1} - \rho_1^{D}D\right) \label{eq:vn}
\end{align}
where $U_{n-1}$ is the mean time to reach state $n$ from state $n-1$.

\subsubsection{Multiple buckets ($K \ge 1$)}

Next, extend  the analysis above for the case of multiple buckets.  We denote by $\bm{p}$ a vector whose $i$-th element equals the  complement of the probability that a sample causes the number of balls at bucket $i$ to increase by 1 unit, $\bm{p}=(p_1, \ldots, p_K)$, i.e., $1-p_i$ is the probability that a sample adds a ball into the $i$-th bucket. 
Let $A_K(\bm{p},D)$ be the mean time to absorption,  accounting for $K$ buckets with depth $D$ each, and starting from the initial state wherein there are 0 balls in bucket 1. Then, 
\begin{align}
    A_K(\bm{p},D) &= V_{D+1} + \sum_{i=2}^K V_{D,i,1} 
\end{align}
where $V_{D,i,j}$ is the mean number of samples to increment the number of balls in bucket $i$ by $D$ units, starting from the state wherein the system has $j$ balls at bucket $i$. %  The expression of  $ V_{D+1,1,0}$ was previously computed, and is given by~\eqref{eq:vn}, 
%\begin{align}
%V_{D+1,1,0} &= V_{D+1} %\\
%&= \frac{ \rho+1}{(1-\rho)\rho^{D+1}} \left(\frac{1-\rho^{D+1}}{1-\rho} - \rho^{D+1} {(D+1)}\right) 
% \end{align}
To derive an expression for $V_{D,i,1}$, we let $U_{j,i}$ be the mean time to increment the number of balls at bucket $i$ by 1 unit, starting from $j+1$ balls. In particular,
\begin{equation}
    U_{j,1} = U_{j+1}
\end{equation}
Then, 
\begin{align}
    V_{D,i,1} &= \sum_{j=0}^{D-1} U_{j,i} \\
   &=  \left( \frac{1+\rho_i}{1-\rho_i} + U_{0,i} \right)  \left(\frac{1-\rho_i^{-D}}{1-\rho_i^{-1}} \right) - D \frac{1+\rho_i}{1-\rho_i}  \label{eq:vdi1}
\end{align}
where
\begin{align}
    U_{0,i} &= \frac{1 + p_i U_{D-1,i-1}}{1-p_i} \\
      U_{j,i} &= \rho_i^{-j} \left( \frac{1+\rho_i}{1-\rho_i} + U_{0,i} \right) - \frac{1+\rho_i}{1-\rho_i},
\end{align}
for $j>0$.

\subsubsection{Special case with two buckets $(K=2)$}
Let $A_2$ be the time to absorption with $K=2$ buckets.   $A_2$ can be expressed as a function of $p_1$, $p_2$ and $D$,
\begin{align}
A_2(p_1,p_2, D)  %V_{D+1,1,0} + V_{D,2,1} \\
&= V_{D+1} + V_{D,2,1} \label{eq:a2p1p2d}
\end{align}
where $V_{D+1}$ is given by~\eqref{eq:vn}, $ V_{D,2,1}$ is given by~\eqref{eq:vdi1},
\begin{align}
U_{0,2} &= \frac{1 + p_2 U_{D}}{1-p_2} \\
   &= \frac{1}{1-p_2} \left(1 + p_2  (\rho_1+1)\frac{\rho_1^{-D-1}-1}{1-\rho_1} \right) % \\
    % &=\frac{1+\rho_1}{\rho_1} \frac{1-\rho_1^{-n}}{1-\rho_1^{-1}} + \rho_1^{-n} ({1+\rho_1^{-1})}  
\end{align}
and
\begin{equation}
    \rho_i = \frac{1}{p_i} -1  
\end{equation}

\subsubsection{Hypothesis testing}

The system administrator continuously considers two alternative hypothesis: 
\begin{enumerate}
    \item null hypothesis $H_0$ corresponding to a situation where there is no attack taking place
    \item alternative hypothesis $H_1$ meaning that the system is under attack.
\end{enumerate}

Then, the key quantities of interest can be defined as a function of $H_0$ and $H_1$.

\begin{definition}
The  mean time until a false alarm under $H_0$ is denoted by $A_K$.  It is given by the mean time to  reach the absorbing state of the Markov chain characterizing the bucket algorithm.
\end{definition}

\begin{definition}
A lower bound on the  time until a true positive  under $H_1$  is denoted by $L$.  Assuming all buckets are initially empty, we let \begin{equation}
    L = KD.
\end{equation}
\end{definition}

\begin{definition}
The probability of false alarm is the probability that an alarm is triggered before an attack,
\begin{equation}
    f = \mathbb{P}(R < T)
\end{equation}
where $R$ is a random variable with mean $A_K$ characterizing the time until an alarm is triggered,  and  $T$ is  a random variable with mean $1/\alpha$ characterizing the time until an attack occurs.
\end{definition}

In this paper, except otherwise noted we assume that $f$ depends on $R$ and $T$ only through their means, i.e., $f = f(A_K, \alpha^{-1})$.

\begin{definition} \label{def:cost}
The expected cost of a given system parameterization is a weighted sum of the probability of false positives, computed under $H_0$,  and a lower bound of the time until detecting an attack, computed under $H_1$,
 \begin{equation}
     C(\bm{p}, w, D, K, \alpha)  =  K D +  w f(A_K, \alpha^{-1})  \label{eq:cost1}
 \end{equation}
\end{definition}

\subsubsection{Modeling the probability of false alarms} 

Let $f$ be the probability of a false alarm.  We consider two distinct models to determine the probability of false alarm as a function of $A_2$:

\begin{enumerate}
    \item \textbf{deterministic model}: under the exponential model, the number of samples taken until a false alarm is approximated as a deterministic distribution with mean $A_2$;
    \item \textbf{exponential model}: under the exponential model, the number of samples taken until a false alarm is approximated as an exponential distribution with mean $A_2$ and rate $1/A_2$;
\end{enumerate}
We denote by $1/\alpha$  the mean time to attack, i.e., $\alpha$ is the mean attack rate.  Then,
\begin{equation}
    f = e^{- A_2 \alpha} \label{eq:fexp1}
\end{equation}
and
\begin{align}
    f = \frac{1/A_2}{\alpha + 1/A_2}  =  \left( 1+{A_2}{\alpha} \right)^{-1} \label{eq:fexp2}
\end{align}
under the deterministic and exponential models, respectively.

\subsubsection{Optimization problem formulation}

Given a target false positive probability, denoted by $F$, the system administrator goal is to  determine the optimal number of buckets and bucket  depth so as to 
minimize the lower bound on number of samples to detect and attack, $L$, while still meeting the target false positive probability. 
\begin{align}
&{\mbox{\sc  Problem with Hard Constraints:}}\quad  \nonumber \\
&    \min \quad L=KD \\ \label{eq:hard}
 &   \textrm{subject to} \quad f(K,D) \leq F 
\end{align}
In what follows, we assume that $K$ is fixed and given.  Then, as $f$ is strictly decreasing with respect to $D$, the constraint above will be always active and the problem translates into finding the minimum value of $D$ satisfying the constraint.  The problem above is similar in spirit to a Neyman-Pearson hypothesis test, for which similar considerations apply, i.e., the optimal parameterization of the test is the one that satisfies a constraint on the false positive probability.  

Alternatively, the problem above can be formulated through the corresponding Lagrangian, 
\begin{align} \label{eq:lag}
&{\mbox{\sc  Problem with Soft Constraints:}}\quad \nonumber  \\
& \min     \mathcal{L}(D) = K D + w (f(K,D)- F)
\end{align}
where $w$ is the Lagrange multiplier.  The Lagrangian naturally leads to an alternative formulation of the problem, wherein  the hard constraint in~\eqref{eq:hard} is replaced by a soft constraint corresponding to the penalty term $f(K,D)- F $ present in the cost Lagrangian. The Lagrangian is a cost function, motivating Definition~\ref{def:cost}. Note that as $wF$ is a constant, minimizing~\eqref{eq:lag} is equivalent to minimizing~\eqref{eq:cost1}.

Note that whereas the {\mbox{\sc  Problem with Hard Constraints}} is defined as a function of the target false alarm probability $F$, the {\mbox{\sc  Problem with Soft Constraints}}   is defined as  a function of the weight $w$.  Although there is a mapping between the two problems, the target false alarm probability may be easier to interpret as it has a concrete physical interpretation as opposed to $w$, which is a Lagrange multiplier.  Nonetheless, the cost function defined by $w$ allows to visually determine the value of $D$ that minimizes cost. For this reason, the two formulations may be complementary, as indicated in the upcoming section through a numerical example parameterized using data from our controlled experiments. 

\toDM{\cg{We should show the results in the analytical model stating that values from 12 to 15 is adequate}
}

\begin{figure}[t]
    \centering
    \includegraphics[width=0.4\textwidth]{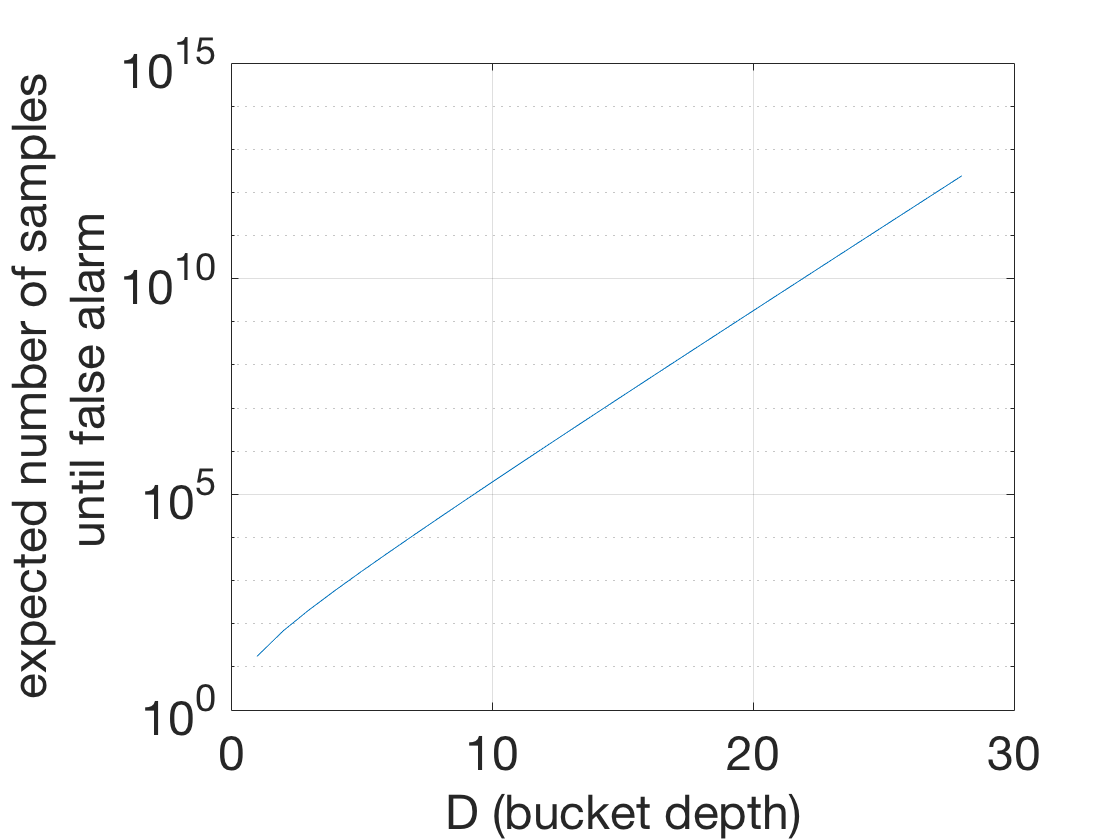}
    \caption{       Expected number of samples until false alarm,  derived from the proposed analytical model.
    We note that   for $D=15$ the number of samples until a false alarm surpasses   $10^7$.} \label{fig:modelpar1}
\end{figure}

\begin{figure}[t]
    \centering
    \includegraphics[width=0.4\textwidth]{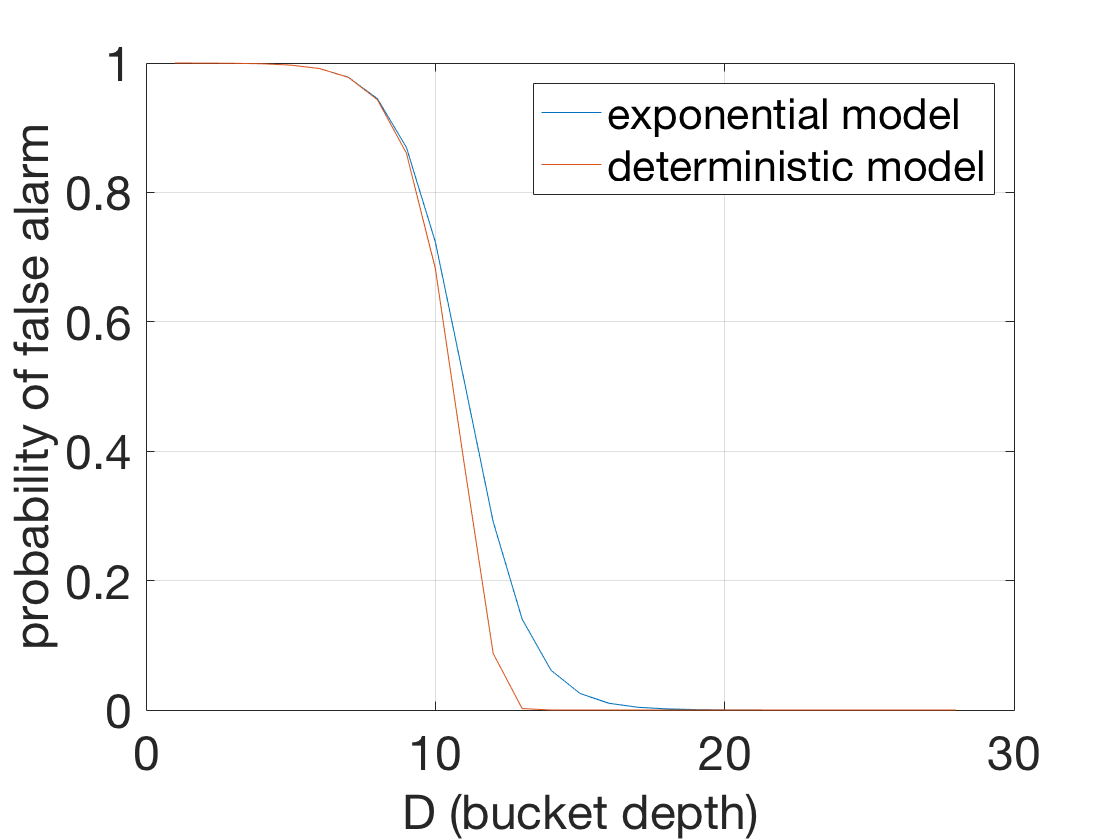}
\caption{ Probability of false alarm, under exponential and deterministic models. In both cases, when $D=15$ the probability of false alarm is already close to 0.}  \label{fig:modelpar2}
\end{figure}

\begin{figure}[t]
    \centering
    \includegraphics[width=0.4\textwidth]{plot4.png}
    \caption{ Cost as a function of bucket depth $(D)$.  Cost is given by $C=w f+ K D$, with $K=2$ and $w=909$, where $f$ is the probability of false alarm. Under the deterministic (resp., exponential) model, cost is minimized for $D=13$ (resp., $D=18$). }
    \label{fig:modelpar3}
\end{figure}

\begin{comment}

\begin{figure}[t]
    \centering
    \includegraphics[width=0.4\textwidth]{bucketfig3.png}
    \caption{ Cost as a function of bucket depth $(D)$.  Cost is given by $C=w f+ K D$, with $K=2$ and $w=909$, where $f$ is the probability of false alarm. Under the deterministic model, cost is minimized for $D=13$. }
    \label{fig:modelpar3}
\end{figure}

\end{comment}

\subsubsection{Experimental results}

Next, our goal is to parameterize the proposed model  from  the experimental results. To that aim, we focus on  the \\ TRADE\_LOOKUP transaction, for which we  identify  that $p_1$ and $p_2$ equal 0.46 and 0.71, respectively. 

Figure~\ref{fig:modelpar1} shows the expected number of samples until false alarm,  derived from the proposed analytical model.
    We note that   for $D=15$ the number of samples until a false alarm surpasses   $10^7$. 
Figure~\ref{fig:modelpar1} is obtained from~\eqref{eq:a2p1p2d}, with  $K=2$, $p_1=0.46$,  $p_2=0.71$, and letting $D$ vary between 1 and 30.

Figures~\ref{fig:modelpar2} and~\ref{fig:modelpar3} account for an attack model, wherein the mean time between  attacks is $1/\alpha=5 \times 10^5$ samples, i.e., the attack rate is  $\alpha=2 \times  10^{-6}$ attacks per sample.   As the bucket depth increases, the probability of false alarm decreases.   When $D=15$, the probability of false alarm is close to 0.

As discussed above, there  is a tradeoff between the probability of false alarm and the time to detect attacks once they occur.  To cope with such a tradeoff, we consider both approaches previously introduced, namely the hard and soft constraint problems.  
Under the hard constraint problem,  a target probability of false alarm is determined, and the minimum value of $D$ that satisfies such target is sought.  For instance, if we set $F=0.03$ then the minimum value of $D$ satisfying the constraint is $D=15$ under the exponential attack model and $D=13$ under the deterministic attack model.

\begin{comment}
a simple cost function, which is given by a weighted sum of two terms.  The first term corresponds to the probability of false alarm  and the second  corresponds to the  number of samples necessary to detect an attack once it occurs,  
\begin{equation}
    C(\bm{p}, w, D, K, \alpha)  = f(A_K, \alpha^{-1}) + w K D
\end{equation}
where $w$ is a weight balancing between the two contending aspects.

\end{comment}

Figure~\ref{fig:modelpar3} shows  $C(\bm{p}, w, D, K, \alpha)$ as  a function of $D$,  letting $K=2$, $p_1=0.46$, $p_2=0.71$ and $\alpha=2 \times  10^{-6}$.  Letting $w=909$, which corresponds to the Lagrange multiplier of the constrained problem under the deterministic model,  the optimal bucket depth equals $D=13$, %.  Considering the same parameterization, the optimal bucket depth equals  $D=18$ under the  exponential model,
which is in agreement with the result  presented in the previous paragraph.  Note that for the exponential model the minimum cost is attained at $D=18$, which is slightly larger than $D=15$ obtained in the previous paragraph. This is because the Lagrange multiplier corresponding to the exponential model is $w=57$.  Using such a smaller weight  favors a reduction in the optimal bucket depth to $D=15$, again in agreement with the results discussed in the previous paragraph.  

% depending on whether the deterministic or exponential   models are used  to determine the probability of false alarm as a function of $A_2$.   

\subsection{Take away message and engineering implications}

\textbf{Reverse engineering utility function of existing systems}  
The results presented in this section are instrumental to reverse engineer the utility function subsumed by existing systems.  For instance, consider a system operating with $K=2$ buckets with depth $D=15$. The analysis presented in the previous section shows that this is optimal, for instance, in case $5\times 10^{5}$ samples are collected inbetween attacks and $w=57$, leading to a false positive probability of roughly 0.03.   Knowing that this is the case, one can tune the utility function, e.g., to account for attacks that occur at different rates, and verify when/if the parameters of the bucket algorithm should be adjusted.

\textbf{Counterfactual analysis} As pointed in the previous paragraph, reverse enginneering the utility function is helpful to perform what if analysis and execute utility-driven model parametrization.  If the system administrator implements global countermeasures against attacks, for instance, it is expected that the rate of attacks will decrease. In that case, the bucket depth can be adjusted accordingly, e.g., using the proposed utility-driven approach presented in this section. The approach can be initially configured through the reverse engineering mechanism previously illustrated, and then tuned to account  for novel system  setups.
k
\begin{comment}

\clearpage
\pagebreak

\begin{figure}[h!]
    \centering
    \includegraphics[width=0.4\textwidth]{bucketfig1.png}
    
       (a) Expected number of samples until false alarm,  derived from the proposed analytical model.
    We note that   for $D=15$ the number of samples until a false alarm surpasses   $10^7$.
    
    \includegraphics[width=0.4\textwidth]{bucketfig2.png}

(b) Probability of false alarm, under exponential and deterministic models. In both cases, when $D=15$ the probability of false alarm is already close to 0.  

    \includegraphics[width=0.4\textwidth]{bucketfig3.png}
    
    (c) Cost as a function of bucket depth $(D)$.  Cost is given by $C=f+0.018 D$, where $f$ is the probability of false alarm. Under the exponential model, cost is minimized for $D=15$. 

    \caption{    Analytical results derived from parameterized model, letting $K=2$, $p_1=0.46$ and $p_2=0.71$. In parts (b) and (c),  we let the attack rate be given by  $\alpha=2 \times  10^{-6}$ attacks per sample. }
    \label{fig:apfig1}
\end{figure}

\end{comment}

\end{appendix}
